# Supplementary material for: Urban Radiance Field Representation with Deformable Neural Mesh Primitives
Source: arXiv:2307.10776 source file (2023-07-20)
Supplement: Supplementary file 1 [file comparison_kitti.tex]

\begin{figure*}[!t]
    \centering
    \includegraphics[width=1\linewidth, trim=0cm 0cm 0cm 0cm, clip]{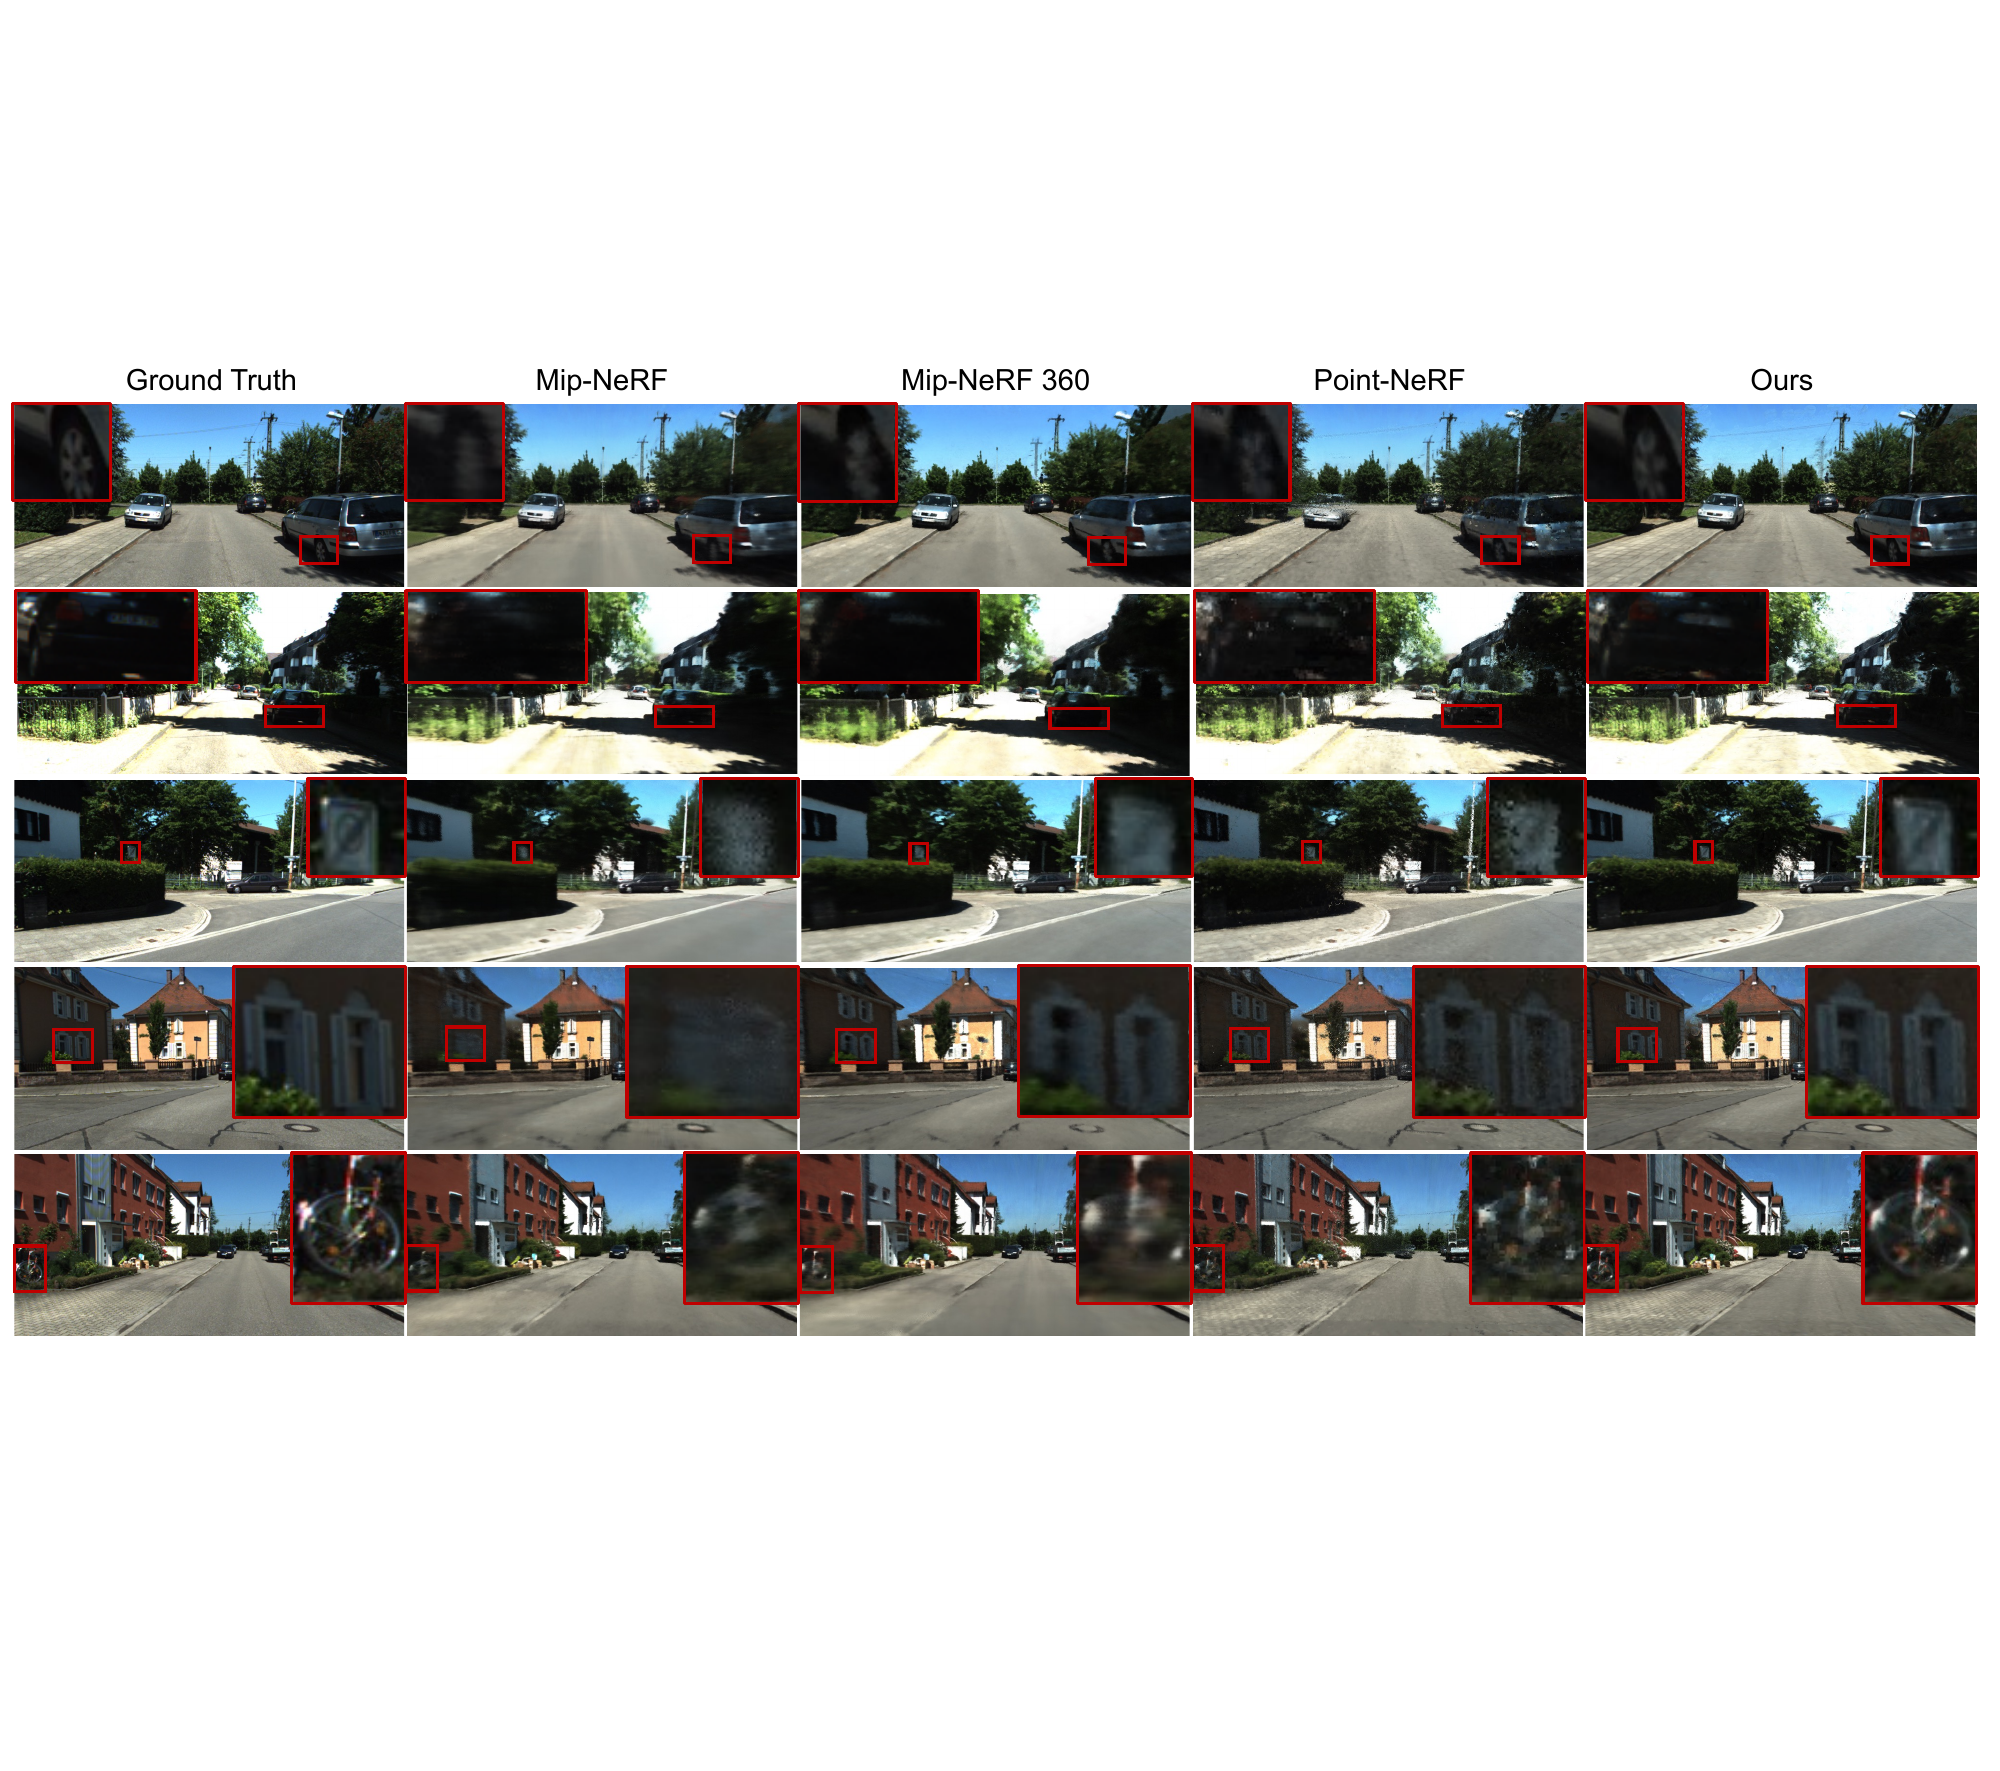}
    \caption{Qualitative comparison of novel view synthesis on KITTI-360 dataset. Cropped patches are scaled to highlight details. Due to the explicit and accurate surface modeling, the proposed method significantly outperforms baseline methods and can effectively recover texture details.}
    \label{fig:comparison_kitti}
\end{figure*}
