# Supplementary material for: Urban Radiance Field Representation with Deformable Neural Mesh Primitives
Source: arXiv:2307.10776 source file (2023-07-20)
Supplement: Supplementary file 3 [file latent_code.tex]

\begin{figure}
\centering
{
 \includegraphics[width=0.95\linewidth]{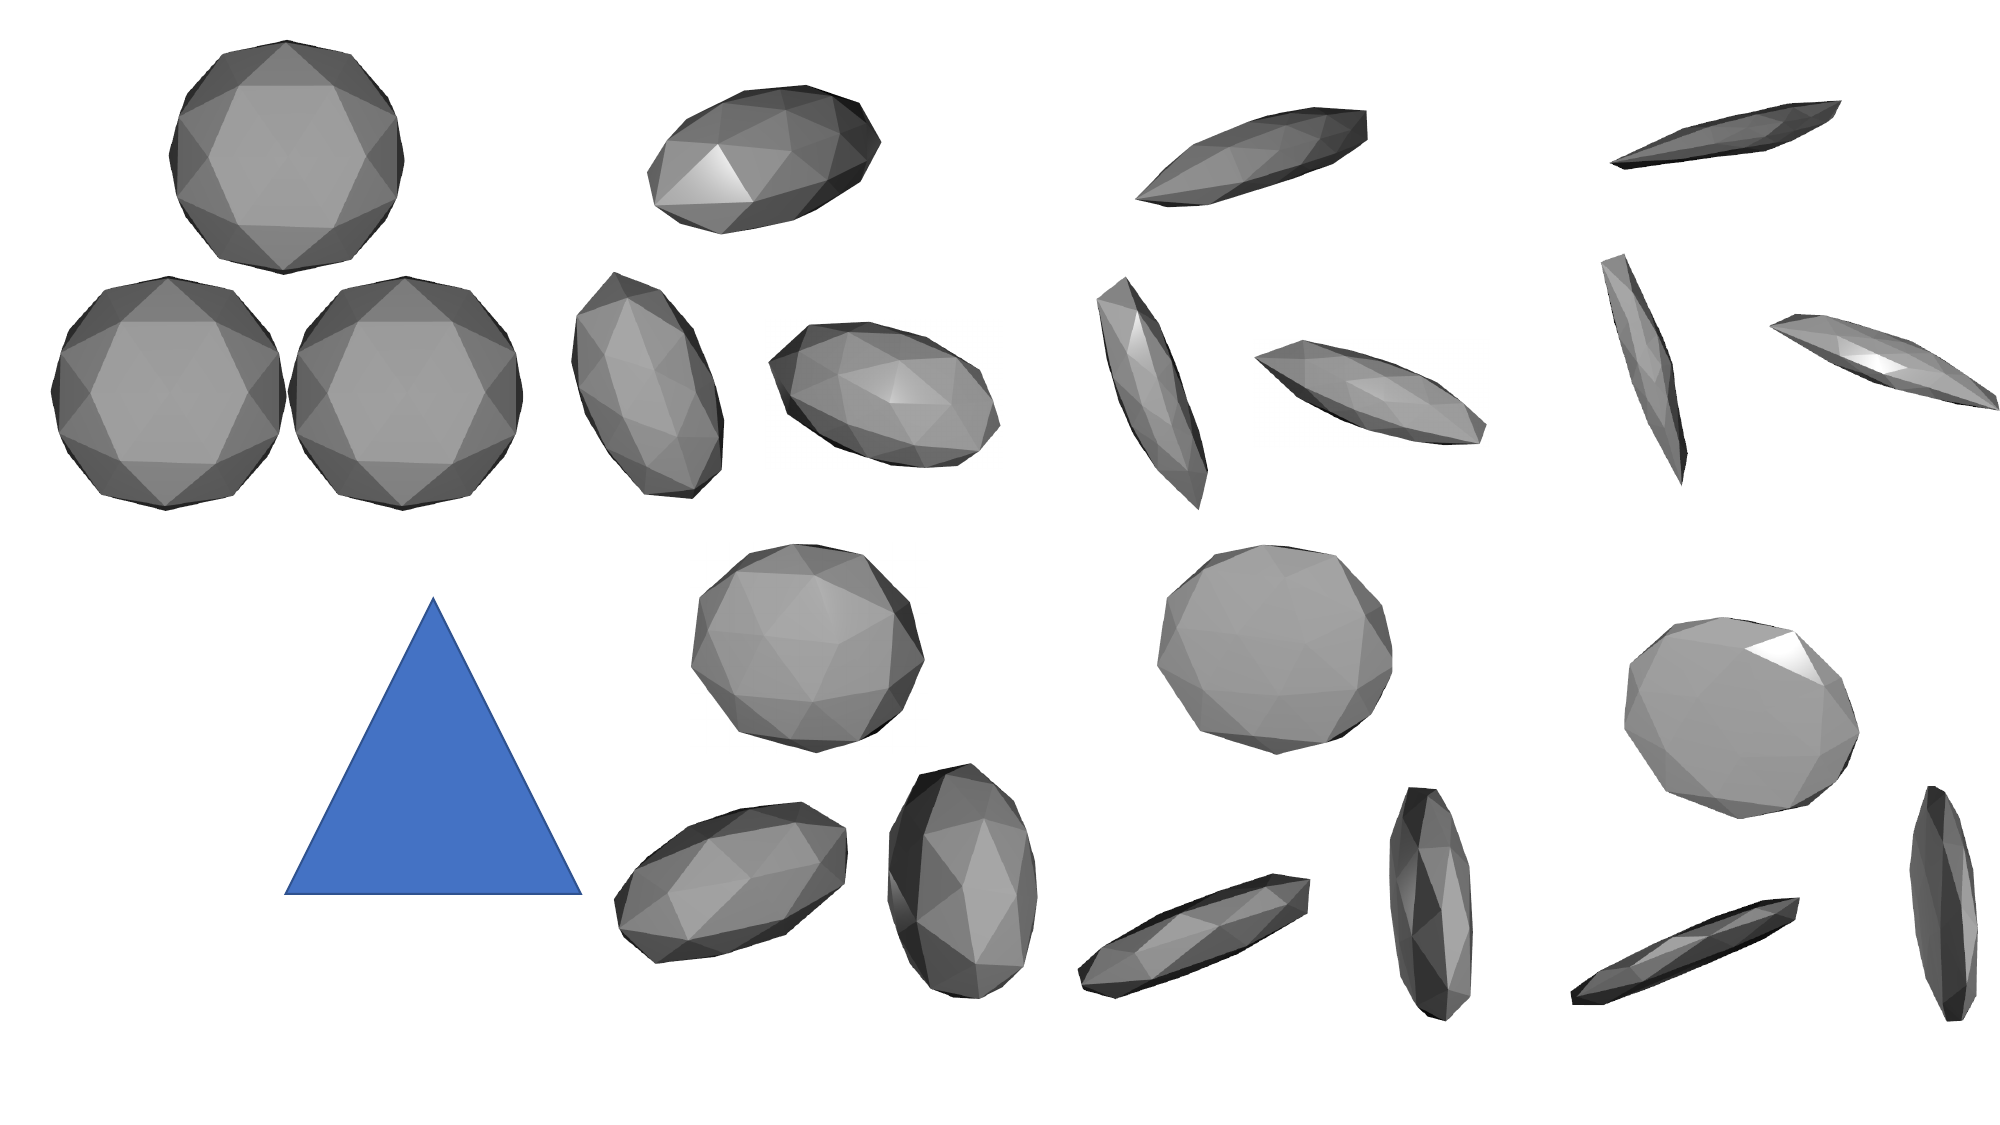}
 }
\caption{Optimization of DNMPs. DNMPs can be deformed from 
spherical template meshes into various basic shapes (\emph{e.g.}, plane, pillar, curved surface, \etc), via optimizing the shape latent codes.}
\label{fig:latent_code}
\end{figure}
