# Supplementary material for: Urban Radiance Field Representation with Deformable Neural Mesh Primitives
Source: arXiv:2307.10776 source file (2023-07-20)
Supplement: Supplementary file 4 [file metashape.tex]

\begin{figure*}[htbp]
    \centering
    \includegraphics[width=1\linewidth, trim=0cm 0cm 0cm 0cm, clip]{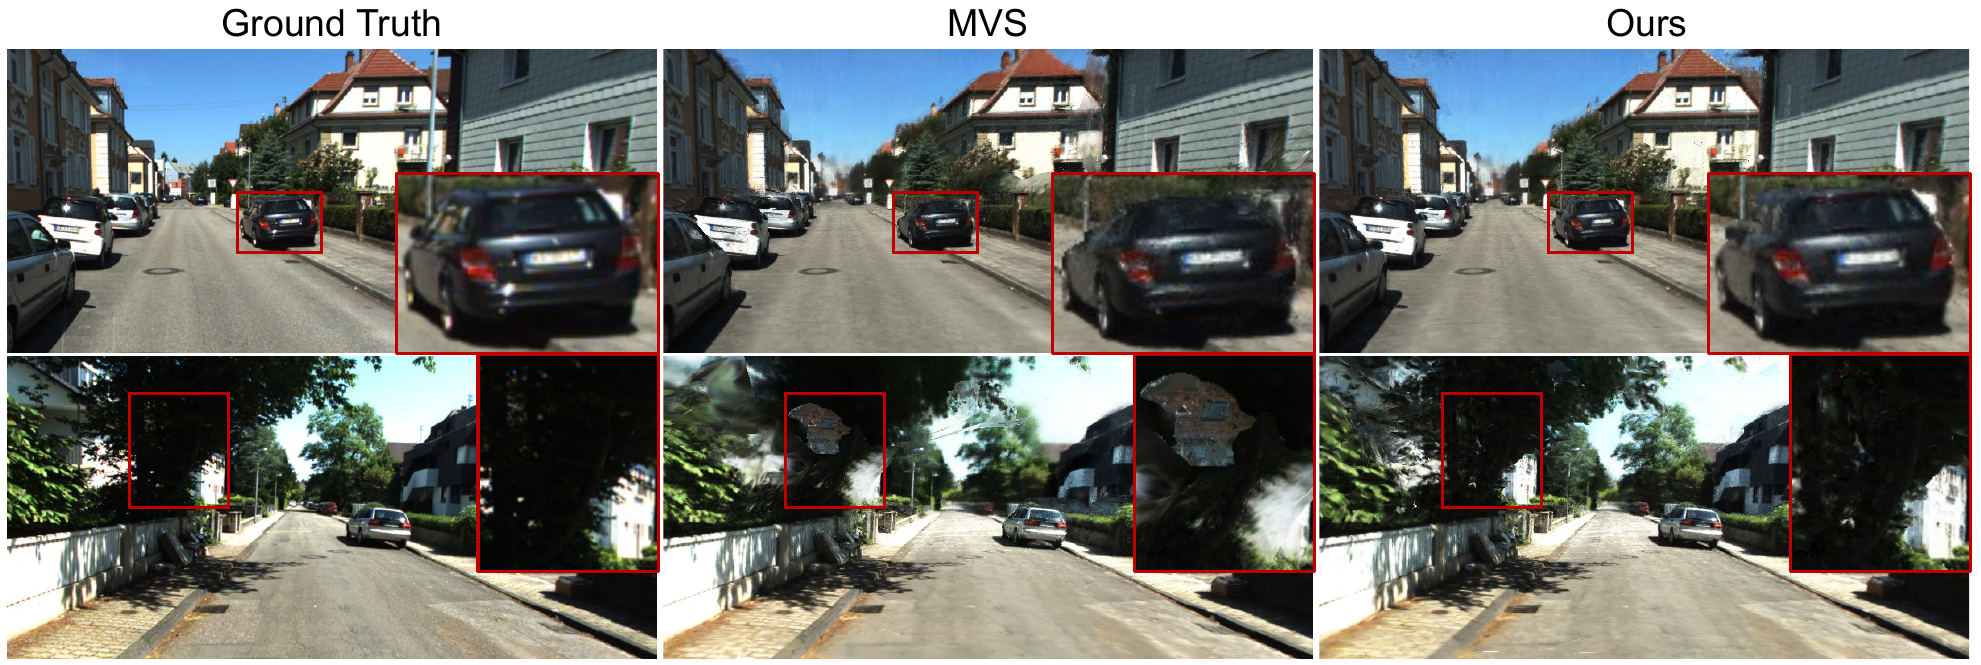}
    % \vspace{-3ex}
    \caption{Qualitative comparison of novel view synthesis on KITTI-360 dataset with neural rendering using meshes reconstructed from Multi-View Stereo (MVS). Cropped patches are scaled to highlight details. Reconstructed meshes from MVS are incomplete (\emph{e.g.}, the upper part of the car in the cropped patches in the first row) and contain occlusions (\emph{e.g.}, the building in the bottom-right corner of the cropped patches in the second row), leading to blurry and unreal rendering results.}
    \label{fig:metashape}
    % \vspace{-3ex}
\end{figure*}
