# Supplementary material for: Urban Radiance Field Representation with Deformable Neural Mesh Primitives
Source: arXiv:2307.10776 source file (2023-07-20)
Supplement: Supplementary file 5 [file primitive_radius.tex]

\begin{figure}
% \resizebox{1.0\linewidth}{!}
\centering
{
 \includegraphics[width=0.95\linewidth]{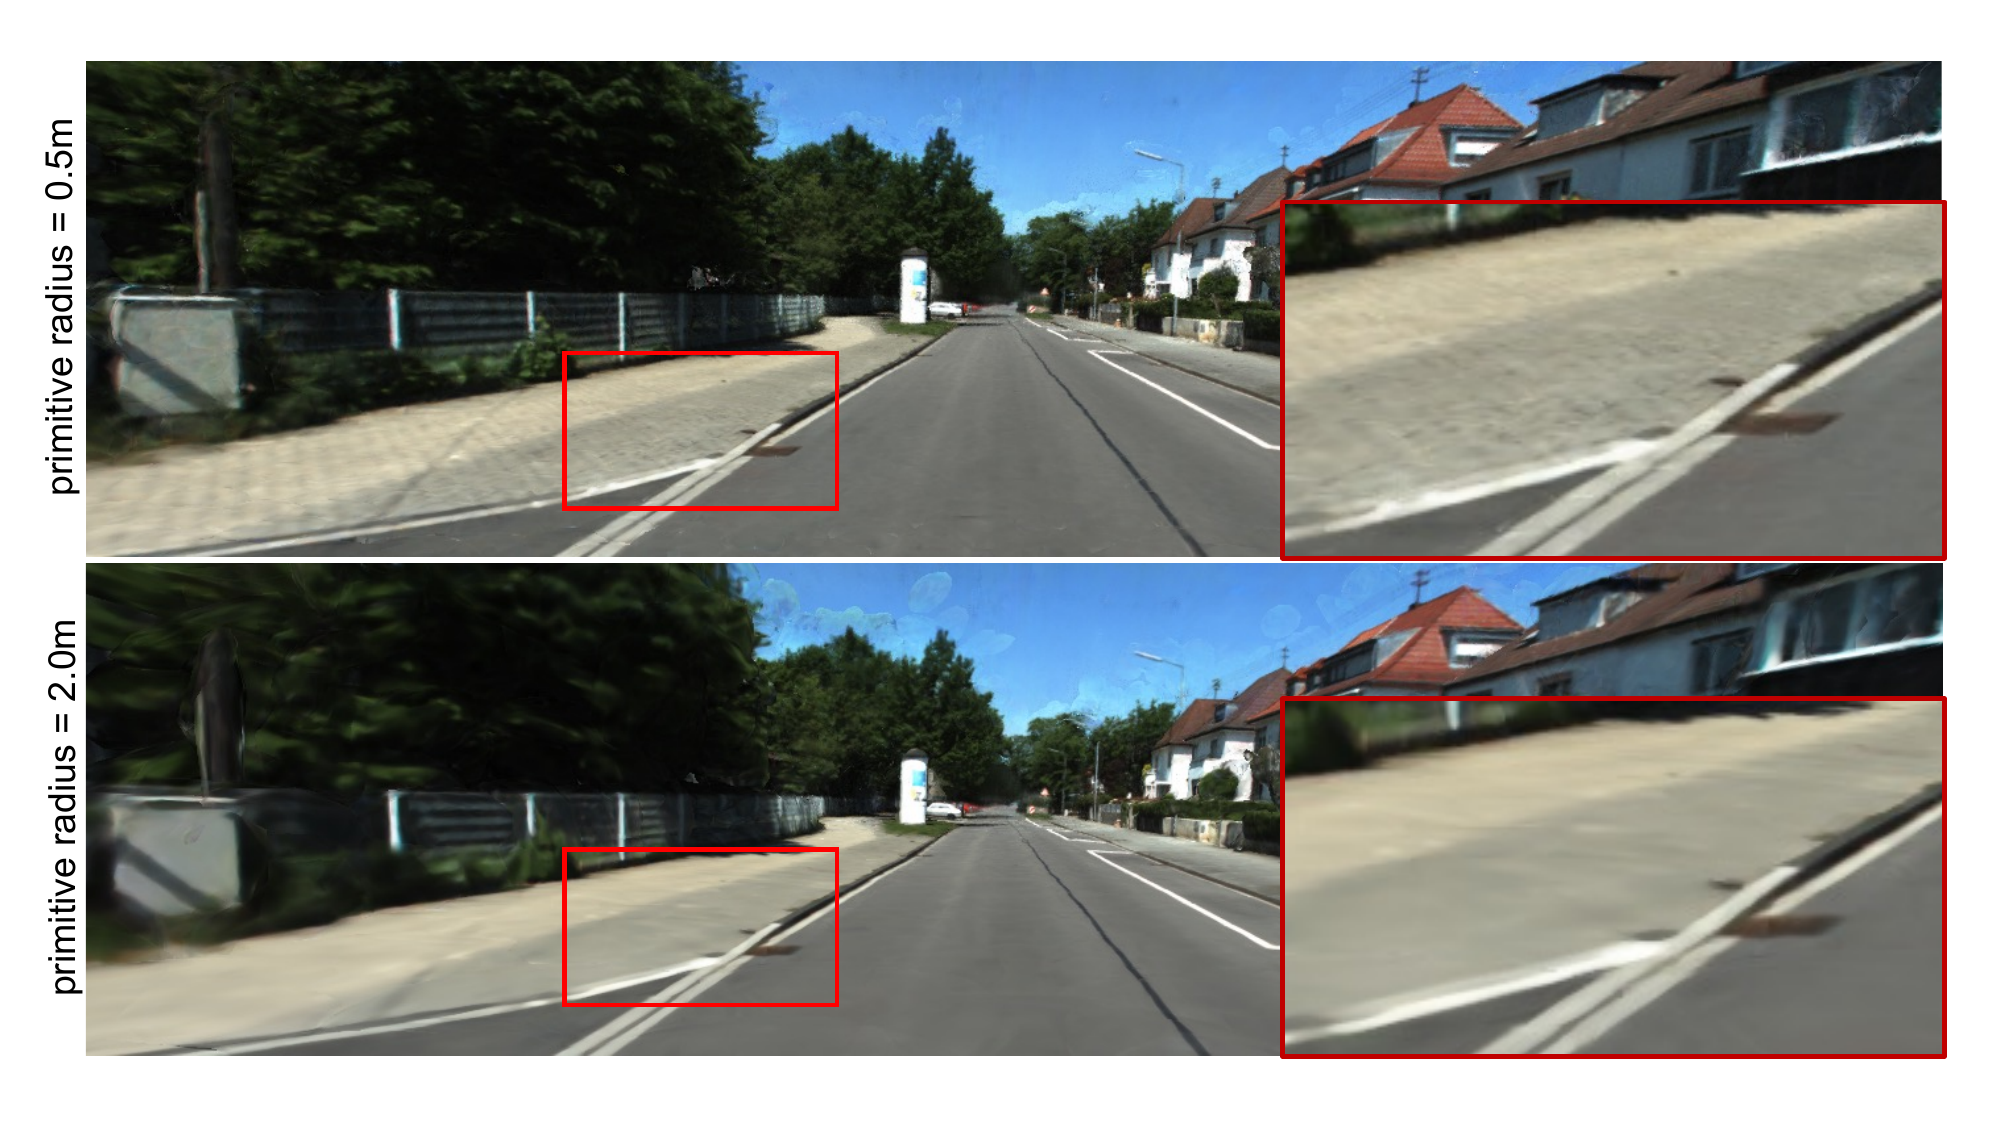}
 }
\caption{View synthesis results based on DNMPs of different sizes. Even only based on the DNMP with a dimension of 2 meters,  the synthesized images are still of acceptable quality,    
though the texture details are lost compared to results of 0.5m-DNMPs.
}
\label{fig:primitive_radius}
\end{figure}
