# Supplementary material for: Urban Radiance Field Representation with Deformable Neural Mesh Primitives
Source: arXiv:2307.10776 source file (2023-07-20)
Supplement: Supplementary file 6 [file scannet.tex]

\begin{figure}[htbp]
\centering
{\includegraphics[width=1.\linewidth]{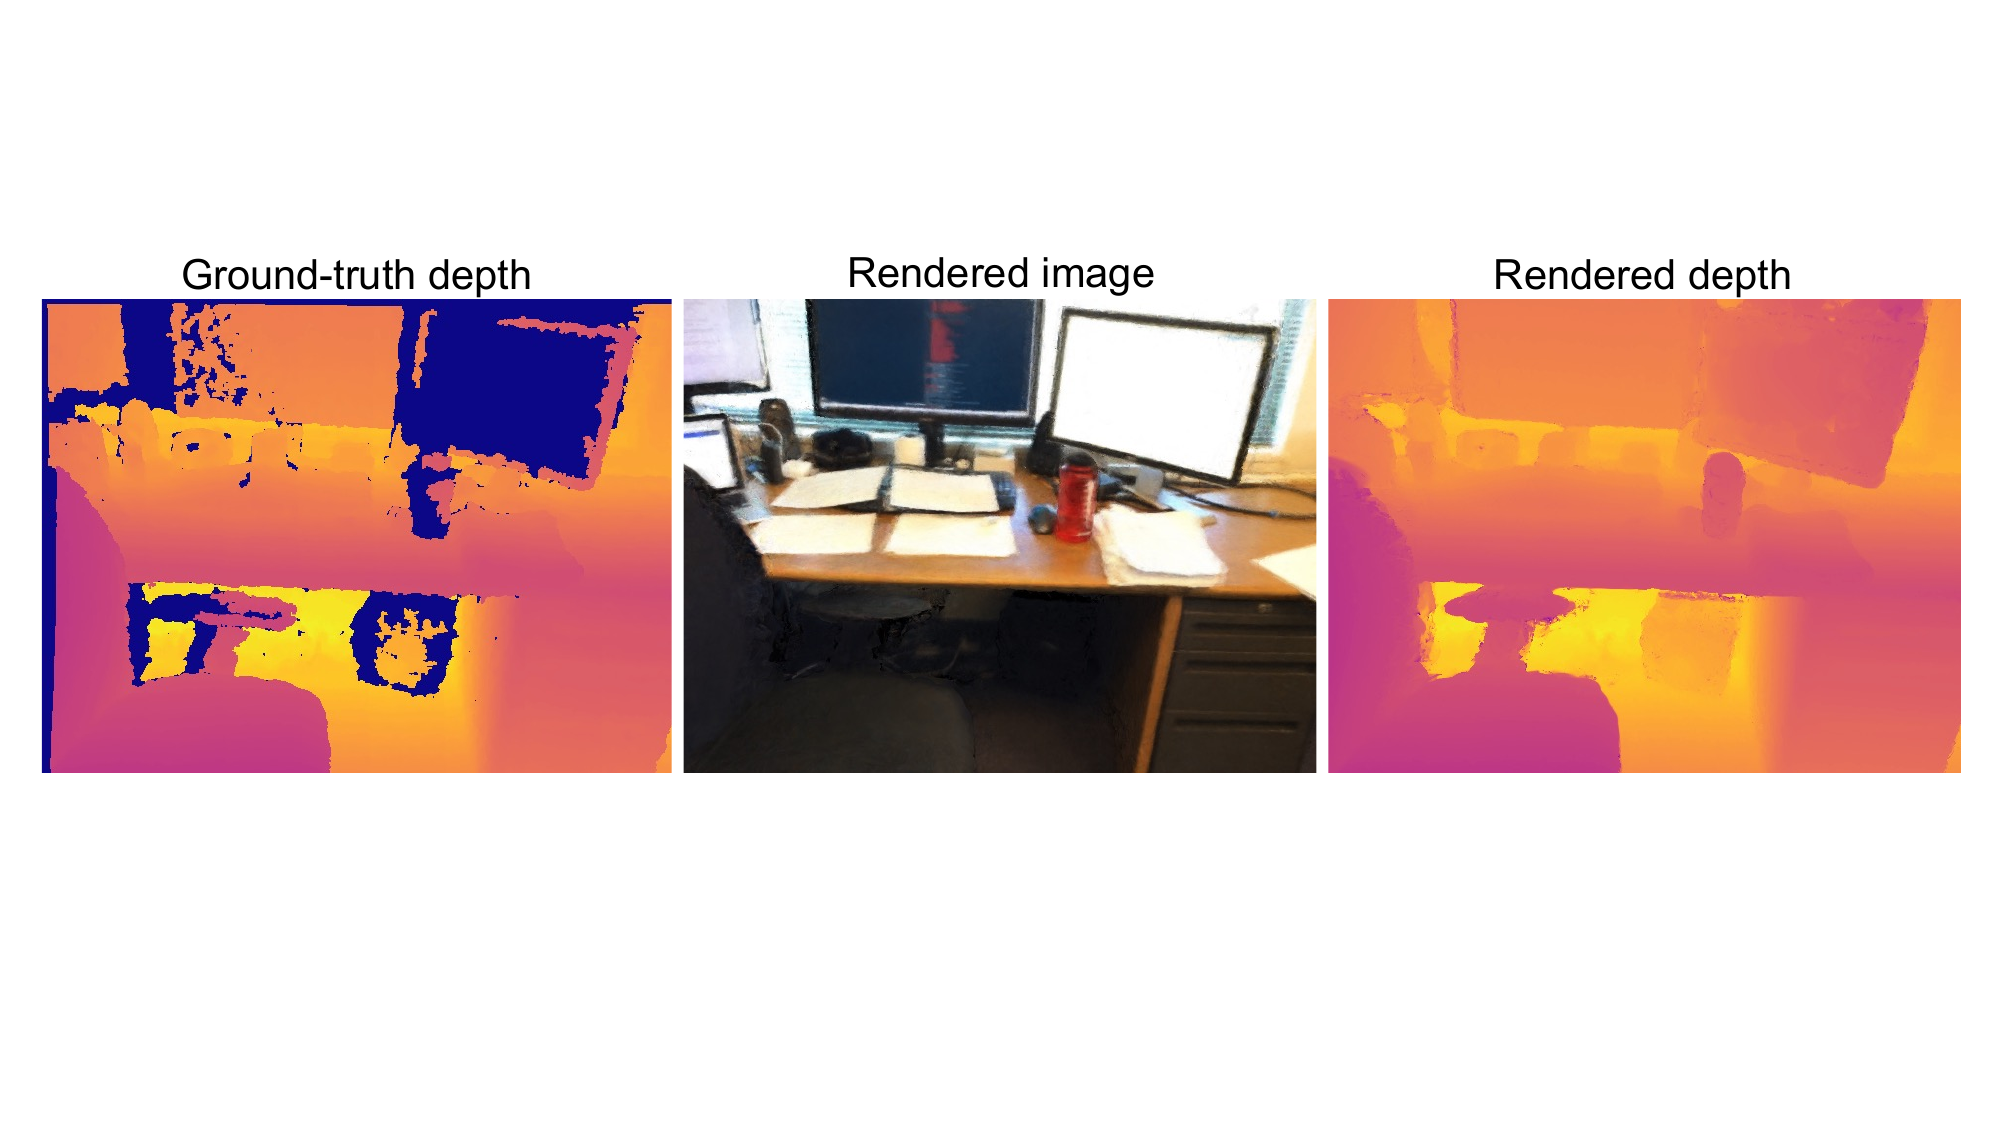}}
\caption{A sample of rendering results on ScanNet dataset.}
\label{fig:scannet}
\end{figure}
