# Supplementary material for: Urban Radiance Field Representation with Deformable Neural Mesh Primitives
Source: arXiv:2307.10776 source file (2023-07-20)
Supplement: Supplementary file 7 [file semantic.tex]

\begin{figure}
\setlength{\abovecaptionskip}{1ex}
 \includegraphics[width=1\linewidth]{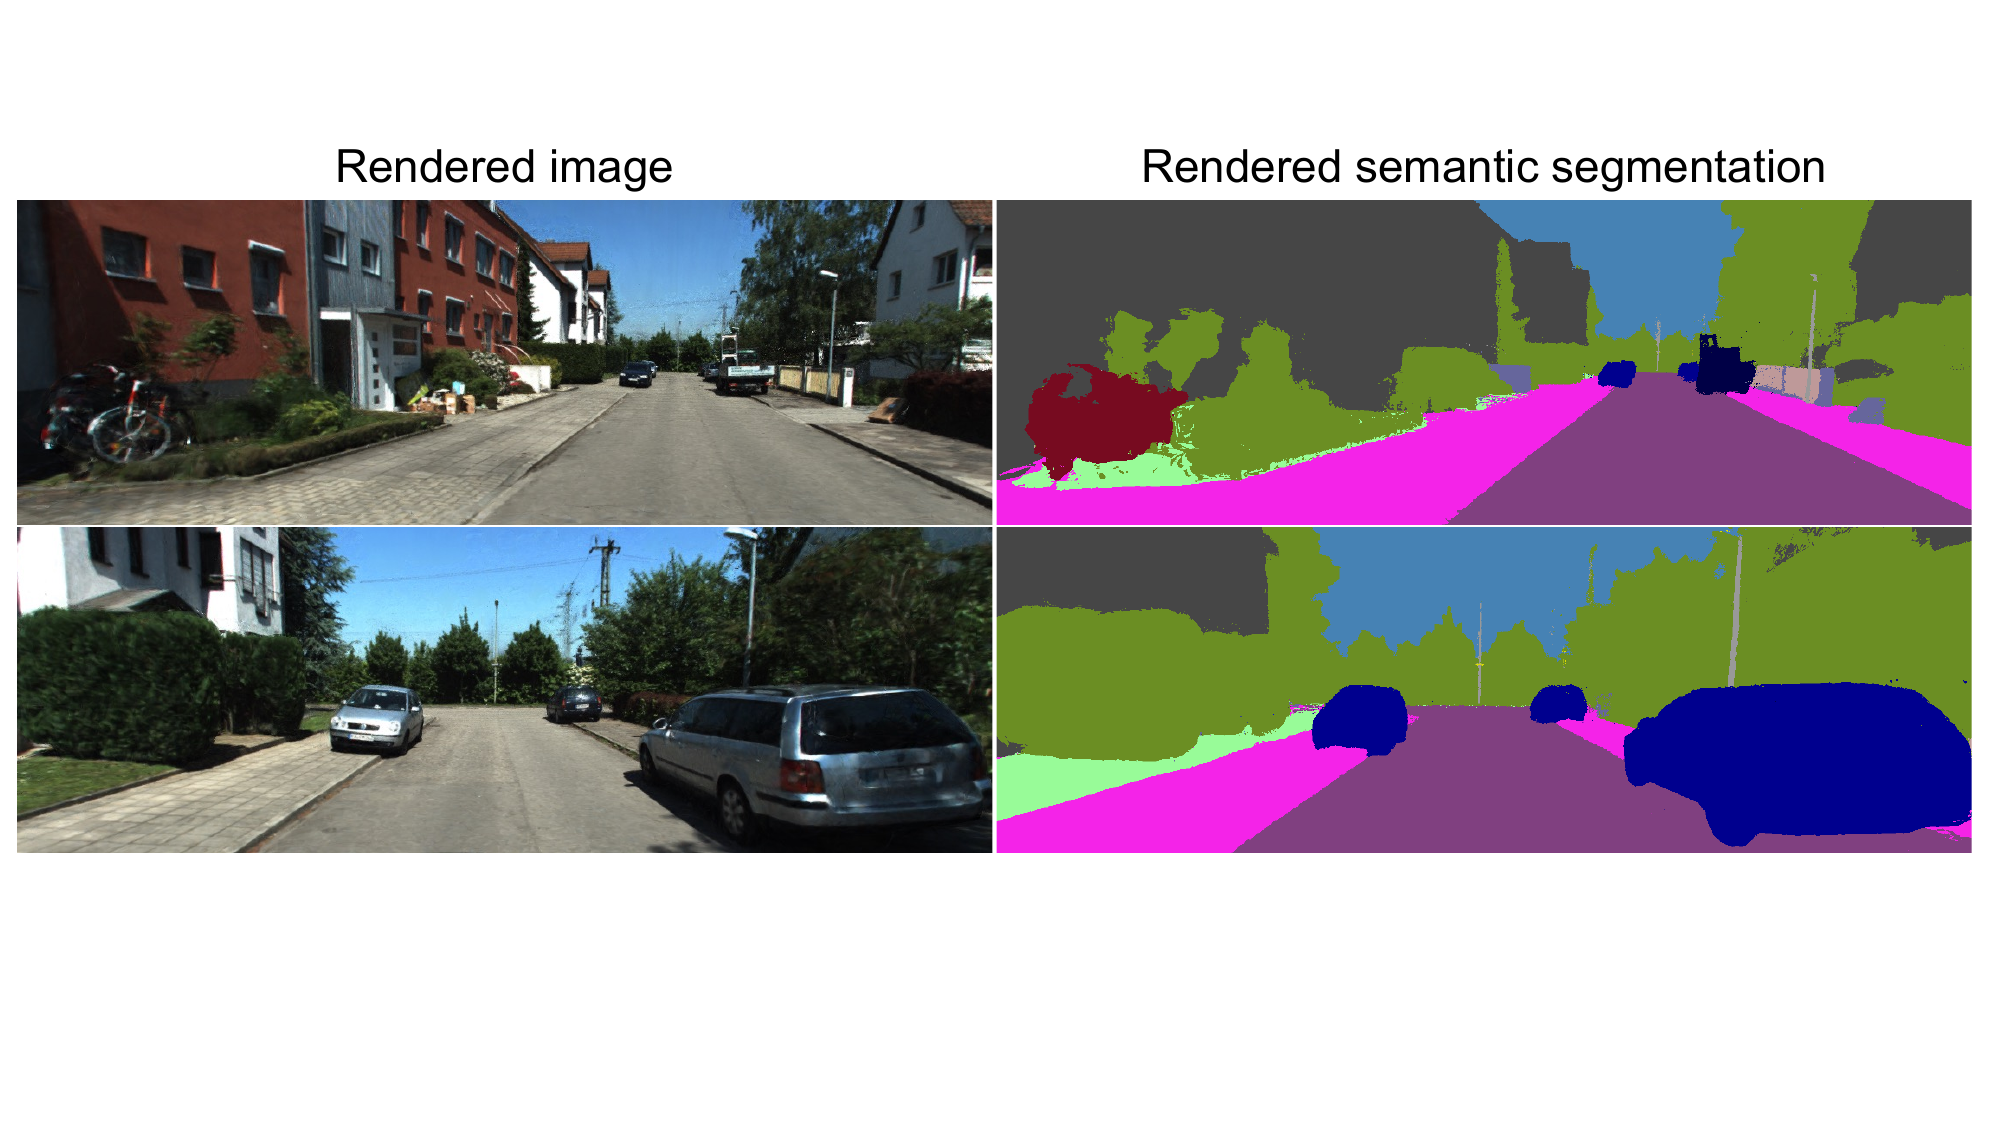}
\caption{Novel semantic synthesis.}
\label{fig:semantic}
\end{figure}
