# Supplementary material for: Urban Radiance Field Representation with Deformable Neural Mesh Primitives
Source: arXiv:2307.10776 source file (2023-07-20)
Supplement: Supplementary file 9 [file comparison_mesh.tex]

\begin{table}[htbp]
\centering
\footnotesize
\caption{
Comparison with neural rendering using meshes reconstructed from Multi-View Stereo (MVS). The comparison is based on KITTI-360 dataset. 
}
\label{tab:comparison_mesh}

\setlength{\tabcolsep}{5mm}{
{
\begin{tabular}{l c c c}
\toprule
\multirow{1}{*}{\textbf{Methods}} & \multicolumn{1}{c}{PSNR$\uparrow$} & \multicolumn{1}{c}{SSIM$\uparrow$} & \multicolumn{1}{c}{LPIPS$\downarrow$}\\
\midrule
MVS~\cite{metashape} & 21.82 & 0.817 & 0.341 \\  
Ours & \textbf{23.41} & \textbf{0.846} & \textbf{0.305} \\  
            
\bottomrule
\end{tabular}
}}
\end{table}
