# Supplementary material for: Urban Radiance Field Representation with Deformable Neural Mesh Primitives
Source: arXiv:2307.10776 source file (2023-07-20)
Supplement: Supplementary file 10 [file comparison_mobile.tex]

\begin{table}[htbp]
\centering
\footnotesize
\caption{
Comparison with MobileNeRF. 
}
\label{tab:comparison_mobile}

\setlength{\tabcolsep}{3mm}{
{
\begin{tabular}{l c c c c}
\toprule
\multicolumn{2}{c}{\textbf{Methods}} & \multicolumn{1}{c}{PSNR$\uparrow$} & \multicolumn{1}{c}{SSIM$\uparrow$} & \multicolumn{1}{c}{LPIPS$\downarrow$}\\
\midrule
\multirow{3}{*}{MobileNeRF} & Stage 1 & 23.18 & 0.823 & 0.350 \\ 
~ & Stage 2 & 22.10 & 0.784 & 0.412 \\ 
~ & Stage 3 & 20.80 & 0.752 & 0.445 \\ 
\midrule
\multicolumn{2}{c}{Ours} & \textbf{23.41} & \textbf{0.846} & \textbf{0.305} \\ 
\bottomrule
\end{tabular}
}}
\end{table}
