# Supplementary material for: Urban Radiance Field Representation with Deformable Neural Mesh Primitives
Source: arXiv:2307.10776 source file (2023-07-20)
Supplement: Supplementary file 11 [file dataset_kitti.tex]

\begin{table}[t]
\centering
% \fontsize{8}{8}\selectfont
\footnotesize
\setlength\tabcolsep{4pt} 

% \caption{Comparison with other competitive methods on KITTI-360 dataset. }
% \caption{Performance comparison of novel view synthesis with other competitive baselines on \texttt{seq\_1}-\texttt{seq\_5} of KITTI-360 dataset.}
\caption{Details of KITTI-360 dataset.}
% \resizebox{\linewidth}{!}
\setlength{\tabcolsep}{7.8mm}{
{
\begin{tabular}{l c c }
\toprule
Sequence & First frame & Last frame\\
\midrule
\texttt{seq\_1} & 715 & 794 \\
\texttt{seq\_2} & 880 & 959 \\
\texttt{seq\_3} & 1102 & 1181 \\
\texttt{seq\_4} & 2170 & 2249 \\
\texttt{seq\_5} & 2900 & 2979 \\
% \rowcolor{Gray}                  
\bottomrule
\end{tabular}
}}
\label{tab:dataset_kitti}
\end{table}
