# Supplementary material for: Urban Radiance Field Representation with Deformable Neural Mesh Primitives
Source: arXiv:2307.10776 source file (2023-07-20)
Supplement: Supplementary file 12 [file dataset_waymo.tex]

\begin{table*}[htbp]
\centering
% \fontsize{8}{8}\selectfont
\footnotesize
\setlength\tabcolsep{4pt} 

\caption{Details of Waymo dataset.}
% \resizebox{\linewidth}{!}
{
\begin{tabular}{l l c c }
\toprule
Set &  Segment Name/ID & First frame & Last frame\\
\midrule
validation 0000 &  segment-10247954040621004675\_2180\_000\_2200\_000\_with\_camera\_labels & 0 & 80 \\
validation 0000 & segment-1071392229495085036\_1844\_790\_1864\_790\_with\_camera\_labels & 135 & 197 \\
validation 0000 &  segment-11037651371539287009\_77\_670\_97\_670\_with\_camera\_labels & 0 & 164 \\
validation 0001 & segment-13469905891836363794\_4429\_660\_4449\_660\_with\_camera\_labels & 0 & 197 \\
validation 0002 & segment-14333744981238305769\_5658\_260\_5678\_260\_with\_camera\_labels & 0 & 198 \\
validation 0002 & segment-14663356589561275673\_935\_195\_955\_195\_with\_camera\_labels & 0 & 197 \\
% \rowcolor{Gray}                  
\bottomrule
\end{tabular}
}
\label{tab:dataset_waymo}
\end{table*}
